# Supplementary material for: Determining the Dielectric Constant of Solid/Liquid Interfaces
Source: arXiv:2406.15964 source file (2024-06-25)
Supplement: Supplementary file 1 [file SI-4.pdf]

Visible ~ 10 μJ/pulse with ~ 75 and 200 $\mu$m spot size, respectively. The angles of incidence were above the critical angle for α-$Al_2O_3$(0001)/water interface to reach Fresnel factor enhancement at total internal reflection (TIR) geometry. The resulting vSFG response was separated from the 800 nm visible beam using a 750 nm short-pass filter (Thorlabs) and collected via a liquid nitrogen cooled (-120 °C) charge-coupled device detector array (Princeton instrument) coupled to a spectrograph (300i Acton Research Corp.)

The non-resonant response of a gold-coated (~100 nm thick) α-$Al_2O_3$(0001) (Team Photon Inc., San Diego, CA, 15 mm x 13 mm x 15 mm) was collected under the PPP polarization configuration for vSFG normalization. After this, the sample spectra were collected in PPP and SSP polarization configurations and then normalized with the spectrum collected from a gold-coated α-$Al_2O_3$(0001) surface.

## II. Experimental geometries:

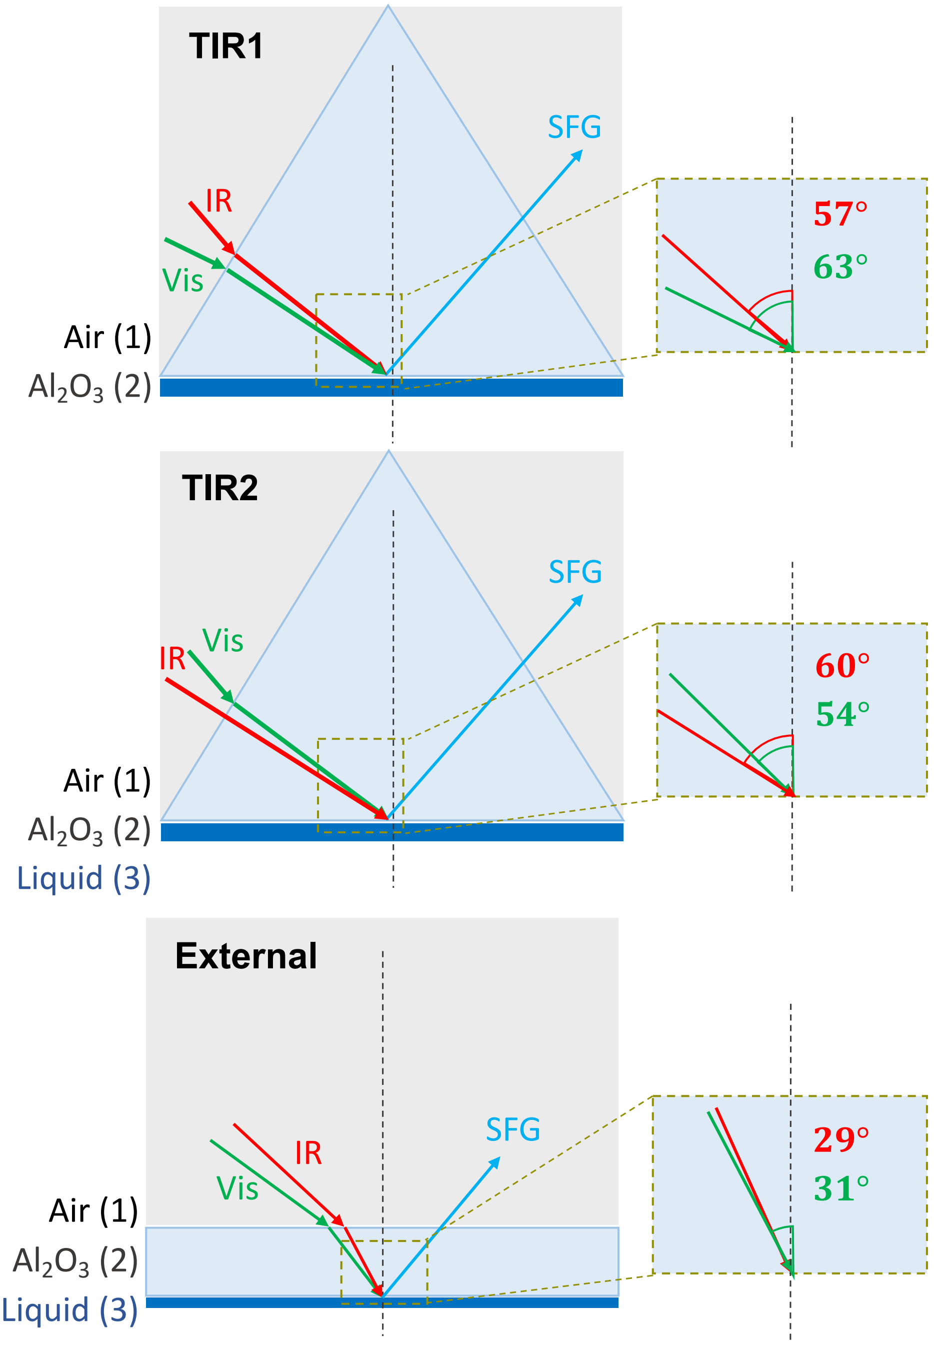


FIG S1: Experimental geometries A) TIR1 geometry vSFG setup at α-$Al_2O_3$(0001)/liquid prism: $\theta_{Vis} \approx 63°, \theta_{IR} \approx 57°$, B) TIR2 geometry vSFG setup at α-$Al_2O_3$(0001)/liquid prism: $\theta_{Vis} \approx 54°, \theta_{IR} \approx 60°$, C) External geometry vSFG setup at liquid/α-$Al_2O_3$(0001) window: $\theta_{Vis} \approx 31°, \theta_{IR} \approx 29°$.

## III. Approaches for deriving the interfacial dielectric constant:

### a. The slab model

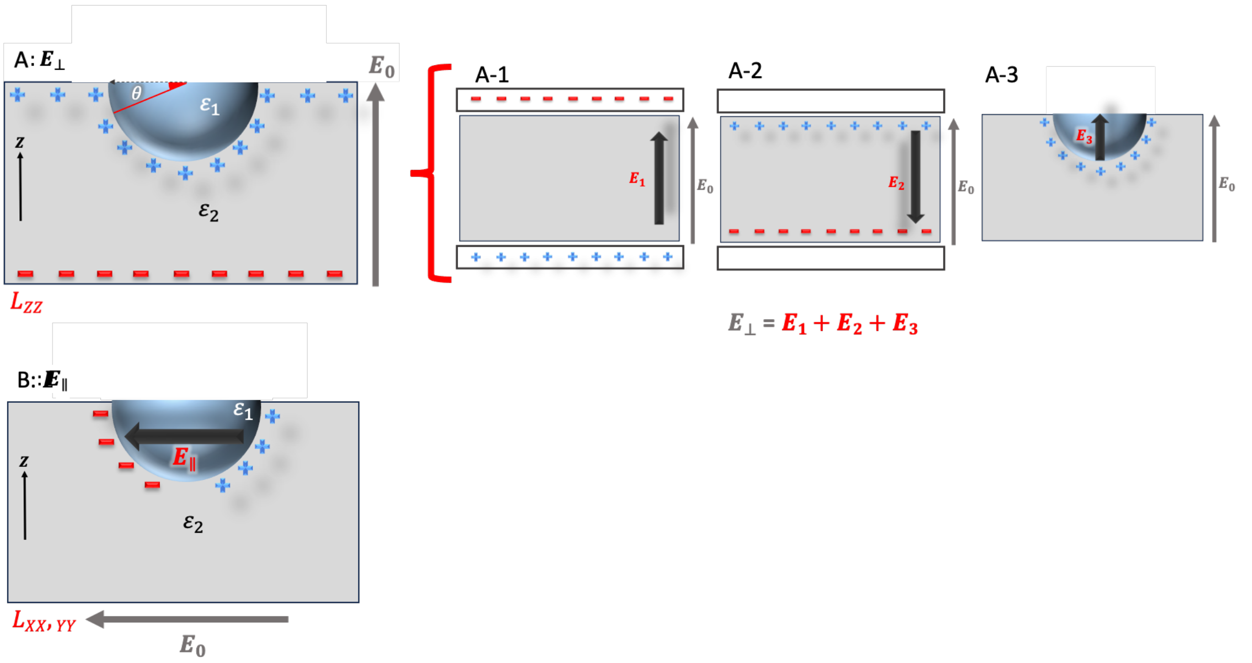


FIG S2: Schematic representation of the resulting electric fields for the slab model for a hemisphere inside a block of a dielectric between the plates of a parallel plate capacitor subjected to an external field along A) the Z-axis (Perpendicular, $E_\perp$) and B) the X or Y-axis (Parallel, $E_{II}$). In case A, the induced field acting on the hemisphere is composed of the components $E_1$ (A-1), $E_2$ (A-2), and $E_3$ (A-3), along the Z-axis. The thick black arrows inside the figures represent the direction of the induced electric field components. The angle θ shown in B is the schematic representation of the angle used in equation S3.

### Induced electric field along the Z-axis: (Perpendicular, $E_\perp$)

To describe the induced electric field along the Z-axis, we considered a block of dielectric (FIG S2 A-1 - A-3: gray box), between the plates of a parallel plate capacitor, polarized by an external electric field ($E_0$) and contains a hemisphere (representing the interfacial molecules with half solvated shells) of different dielectric constant [1]. In this configuration, the induced electric field along the Z-axis (FIG S2A) can be divided into three distinct components considering Gauss's law for a dialectic medium:

$E_1$ (Equation S1, FIG S2 A-1) represents the field due to the charge density on the dielectric plates within the finite interfacial region on the parallel plate capacitor [1].

$$E_1 = \frac{D}{\varepsilon_0} \quad \text{and} \quad D = P + \varepsilon_0 E_0 \qquad \text{then:} \quad E_1 = \frac{P+\varepsilon_0 E_0}{\varepsilon_0} = E_0 + \frac{P}{\varepsilon_0} \tag{S1}$$

$E_2$ (Equation S2, FIG S2 A-2) describes the field due to the charge density induced on the two sides of the dielectric plates in response to $E_1$.

$$E_2 = -\frac{P}{\varepsilon_0} \tag{S2}$$

$E_3$ (Equation S3, FIG S2 A-3) represents the field due to polarization charges on the surface of the hemisphere induced by an external electric field [1].

$$E_3 = \int dE_3 = \frac{-P}{4\varepsilon_0}\int_0^{\pi} \cos^2\theta \sin\theta \, d\theta$$

if $z = \text{Cos}\theta$ then: $dz = -\sin\theta d\theta$

θ represents the polar angle relative to the polarization direction as shown in FIG S2B.

$$E_3 = \int dE_3 = \frac{P}{4\varepsilon_0}\int_1^{-1} z^2 dz = \frac{P}{4\varepsilon_0}\left[\frac{z^3}{3}\right]_1^{-1} = \frac{P}{6\varepsilon_0}$$

Hence: $$E_3 = \frac{P}{6\varepsilon_0} \tag{S3}$$

$$E_\perp = E_1 + E_2 + E_3 = E_0 + \frac{P}{\varepsilon_0} - \frac{P}{\varepsilon_0} + \frac{P}{6\varepsilon_0}$$

We should note that the induced polarization at the surface of the hemisphere will result from the combination of two polarizations with opposite signs due to the difference in permittivity ($\varepsilon_2 \neq \varepsilon_1$). The internal filed which yield an opposite polarization can be calculated by $4\pi P/6$, for a hemisphere using the internal field for non-polar dielectrics [1]. Then we can define $P_1 = (\varepsilon_1 - 1) E_0$ .

Thus: $P = \sum P_i = P_2 - P_1 = \sum E_0\varepsilon_0\,[(\varepsilon_i - 1)] = E_0\varepsilon_0\,[(\varepsilon_2 - 1) - (\varepsilon_1 - 1)]$ then:

$$E_\perp = E_0 + \frac{E_0\varepsilon_0(\varepsilon_2 - \varepsilon_1)}{6\varepsilon_0} = E_0\left(\frac{\varepsilon_2 - \varepsilon_1 + 6}{6}\right) \quad \text{(S4)}$$

In equations S1-S4, the $E_i$ represent the electric fields, $D$ stands for the electric displacement, $P$ denotes the polarization, and $\varepsilon_0$, $\varepsilon_1$ and $\varepsilon_2$ correspond to the dielectric functions in the vacuum, medium 1, and medium 2, respectively.

**Parallel electric field along the XX and YY axes: ($E_\parallel$):**

To calculate the parallel electric filed one may use a dielectric sphere ($\varepsilon_2$) in an infinite dielectric ($\varepsilon_1$) of different dielectric constant [1]. Outside the sphere, without free charge, the potential is going to satisfy the Laplace's equation ( $\nabla^2\varphi = 0$ ) when an external electric field $E_{external}$ has been applied. The analysis involves the utilization of the Laplace equation to compute the electric field both outside ($\varphi_1$) and inside ($\varphi_2$) the hemisphere as follows [1]:

$$\varphi_1 = \sum_{n=0}^{\infty}\left(A_n r^n + \frac{B_n}{r^{n+1}}\right)P_n(cos\theta) \quad \text{(S5)}$$

$$\varphi_2 = \sum_{n=0}^{\infty}\left(C_n r^n + \frac{D_n}{r^{n+1}}\right)P_n(cos\theta) \quad \text{(S6)}$$

Where the $P_n(cos\theta)$ is the spherical harmonics function. When considering the locality, continuity and non-singularity of the electric potential, we can get:

$$\varphi_1|r \to \infty = -E_{external}rcos\theta \quad \text{(S7-1)}$$

$$\varphi_2|r \to 0 = constant\ (nonsingular) \quad \text{(S7-2)}$$

$$\varepsilon_2\frac{\partial\varphi_1}{\partial x}\Big|r \to a = \varepsilon_1\frac{\partial\varphi_2}{\partial x}\Big|r \to a \quad \text{(S7-3)}$$

$$\varphi_1|r \to a = \varphi_2|r \to a \quad \text{(S7-4)}$$

Where a is the radius of the molecular cavity in Lorentz model, and $\varepsilon_1$ and $\varepsilon_2$ are the dielectric constant for medium 1 (hemisphere) and medium 2 (plate), respectively. It is easy to get $B_n = 0$ and $C_n = 0$ when $n \neq 1$ and the solution can be given as:

$$\varphi_1 = \left(\frac{\varepsilon_{12}-\varepsilon_2}{2\varepsilon_1+\varepsilon_2}\frac{a^3}{r^3} - 1\right) E_{external} rcos\theta \qquad \text{(S8-1)}$$

$$\varphi_2 = -\left(\frac{3\varepsilon_1}{2\varepsilon_1+\varepsilon_2}\right) E_{external} rcos\theta \qquad \text{(S8-2)}$$

If we ignore the contribution from the driving electric field $-E_{external} rcos\theta$, then we can get the electric potential generated by surface bounded charge of polarized medium.

$$\varphi_1' = \left(\frac{\varepsilon_2-\varepsilon_1}{2\varepsilon_1+\varepsilon_2}\frac{a^3}{r^3}\right) E_{external} rcos\theta \qquad \text{(S9-1)}$$

$$\varphi_2' = -\left(\frac{\varepsilon_1-\varepsilon_2}{2\varepsilon_1+\varepsilon_2}\right) E_{external} rcos\theta \qquad \text{(S9-2)}$$

Then the electric field generated by surface bounded charge ($E_0$ and $E_0{}'$) can be given as:

$$E_{inside} = -\nabla\varphi_2 = \frac{3\varepsilon_1}{2\varepsilon_1+\varepsilon_2} E_{external} \qquad \text{(S10-1)e}$$

$$E_{outside}{}' = -\nabla\varphi_1' = -\nabla\varphi_2' = \frac{\varepsilon_2-\varepsilon_1}{2\varepsilon_2+\varepsilon_1} E_{external} \qquad \text{(S10-2)}$$

In this scenario we consider the $E_{external} = E_{\parallel}$ and $E_{inside} = E_0$ as a driving force for the induced polarization outside the hemisphere (FIG S2 B).

$$E_{\parallel} = E_0 \left(\frac{2\varepsilon_2+\varepsilon_1}{3\varepsilon_2}\right) \qquad \text{(S11)}$$

Considering this scenario the induced electric field is described with similar approach to Shen et.al while considering $\varepsilon_1 = 1$ the parallel electric filed will reduce to the $E_{\parallel} = E_0 \left(\frac{2\varepsilon_2+1}{3\varepsilon_2}\right)$ [2].

The perpendicular ($E_{\perp}$: FIG S2A) and parallel ($E_{\parallel}$: FIG S2B) and electric field components (as explained above along the X or Y-axis and the Z-axis, respectively) at the interface can be determined using the Fresnel equations (equations S12-1 – S12-3) [3].

$$L_{XX}(\omega_I) = \frac{2\varepsilon_1(\omega_I)\cos\gamma_I}{\varepsilon_1(\omega_i)\cos\gamma_I + \varepsilon_2(\omega_I)\cos\theta_I} \quad \text{(S12 − 1)}$$

$$L_{YY}(\omega_I) = \frac{2\varepsilon_1(\omega_I)\cos\theta_I}{\varepsilon_1(\omega_I)\cos\theta_I + \varepsilon_2(\omega_I)\cos\gamma_I} \quad \text{(S12 − 2)}$$

$$L_{ZZ}(\omega_I) = \frac{2\varepsilon_2(\omega_I)\cos\theta_I}{\varepsilon_1(\omega_I)\cos\gamma_I + \varepsilon_2(\omega_I)\cos\theta_I}\frac{\varepsilon_1(\omega_I)}{\varepsilon'(\omega_I)} \quad \text{(S12 − 3)}$$

Knowing that $L_{ZZ}/L_{YY} = \varepsilon_1/\varepsilon'$, $L_{XX} = L_{YY} = E_{\perp}/E_0$ and $L_{ZZ} = E_{\parallel}/E_0$ we have [2]:

$$\frac{L_{zz}}{L_{xx}\ or\ L_{yy}} = \frac{E_{\parallel}}{E_{\perp}} = \frac{\varepsilon_1}{\varepsilon'} = \frac{\left(\frac{2\varepsilon_2+\varepsilon_1}{3\varepsilon_2}\right)}{\left(\frac{\varepsilon_2-\varepsilon_1+6}{6}\right)} = \frac{2(2\varepsilon_2+\varepsilon_1)}{\varepsilon_2(\varepsilon_2-\varepsilon_1+6)} \quad \text{(S13)}$$

Thus, by simplifying and reordering equation S13 we would have:

$$\varepsilon' = \frac{\varepsilon_1\varepsilon_2(\varepsilon_2-\varepsilon_1+6)}{2(2\varepsilon_2+\varepsilon_1)} \quad \text{(S14)}$$

knowing $n = \sqrt{\varepsilon}$

$$n' = \sqrt{\frac{{n_1}^2\,{n_2}^2({n_2}^2-{n_1}^2+6)}{2(2{n_2}^2+{n_1}^2)}} \quad \text{(S15)}$$

**b.** The Lorentz model

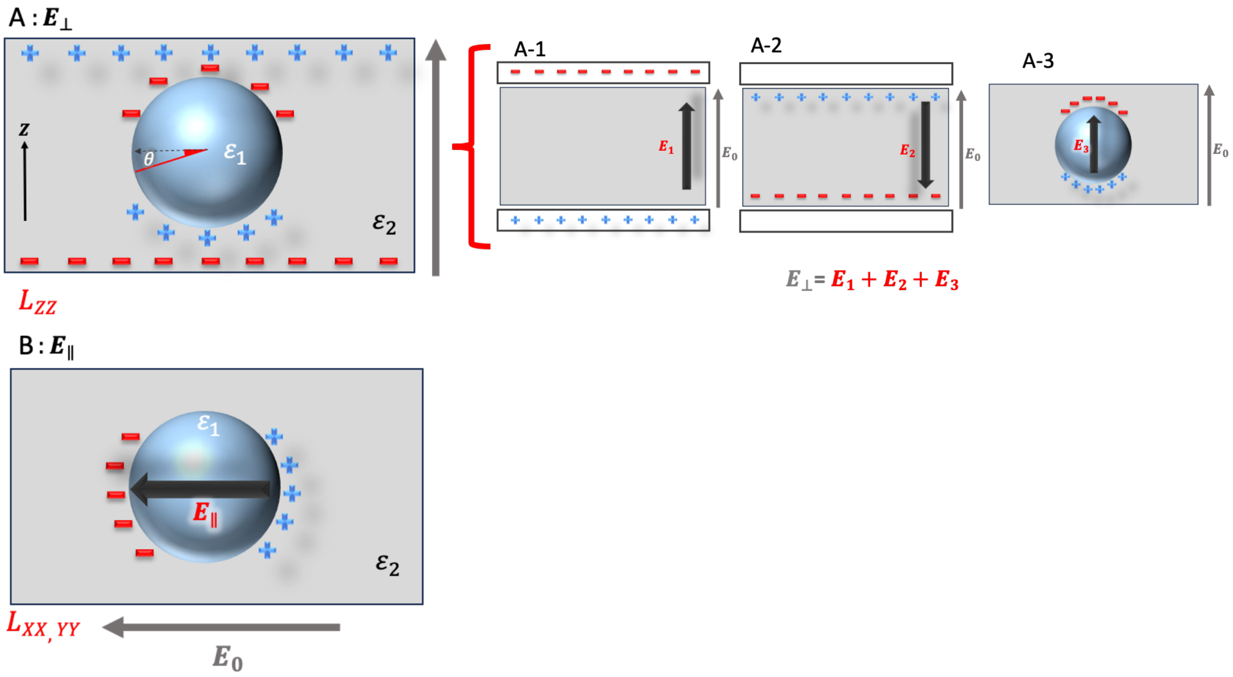


FIG S3: Schematic representation of the resulting electric fields for the Lorentz model for a sphere inside block of dielectric between the plates of a parallel plate capacitor subjected to an external field along A) the Z-axis (Perpendicular, $E_{\perp}$) and B) the X or Y-axis (Parallel, $E_{II}$). In case A, the induced field acting on the sphere is composed of the components $E_1$ (A-1), $E_2$ (A-2), and $E_3$ (A-3), along the Z-axis. The thick black arrows inside the figures represent the direction of the induced electric field components. The angle θ shown in B is the schematic representation of the angle used in the equation S18.

**Electric field along the Z-axis: (Perpendicular, $E_{\perp}$)**

Unlike the half-solvated sphere, here the entire sphere is immersed in the dielectric medium and is considered fully solvated. In this configuration, similar to the hemisphere approach, the induced electric field along the Z-axis comprises three distinct components:

$E_1$ (Equation S16, FIG S3 A-1) characterizes the field arising from the charge density on the dielectric plates within the finite interfacial area on the parallel plate capacitor.

$$E_1 = \frac{D}{\varepsilon_0} \quad \text{and} \quad D = P + \varepsilon_0 E_0 \qquad \text{then:} \quad E_1 = \frac{P+\varepsilon_0 E_0}{\varepsilon_0} = E_0 + \frac{P}{\varepsilon_0} \tag{S16}$$

$E_2$ (Equation 17, FIG S3 A-2) represents the field resulting from the charge density induced on both sides of the dielectric plates due to $E_1$.

$$E_2 = -\frac{P}{\varepsilon_0} \quad \text{(S17)}$$

$E_3$ (Equation S18, FIG S3 A-3) represents the field intensity due induced polarization charges on the surface of the sphere by an external electric field.

$$E_3 = \int dE_3 = \frac{-P}{2\varepsilon_0}\int_0^{\pi} \cos^2\theta \sin\theta \, d\theta, \text{ if } z = \text{Cos}\theta; \text{ Then } dz = -\sin\theta d\theta$$

$$E_3 = \int dE_3 = \frac{-P}{2\varepsilon_0}\int_0^{\pi} \cos^2\theta \sin\theta \, d\theta$$

if $z = \text{Cos}\theta$ then: $dz = -\sin\theta d\theta$

θ represents the polar angle relative to the polarization direction as shown in FIG S2B.

$$E_3 = \int dE_3 = \frac{P}{2\varepsilon_0}\int_1^{-1} z^2 dz = \frac{P}{42}\left[\frac{z^3}{3}\right]_1^{-1} = \frac{P}{2\varepsilon_0}$$

Hence: $$E_3 = \frac{P}{3\varepsilon_0} \quad \text{( S18)}$$

$$E_\perp = E_1 + E_2 + E_3 = E_0 + \frac{P}{\varepsilon_0} - \frac{P}{\varepsilon_0} + \frac{P}{3\varepsilon_0}$$

Knowing that $P = E_0\varepsilon_0\,[(\varepsilon_i - 1)]$ and similar to the scenario we explained above then:

$$E_\perp = E_0 + \frac{E_0\,\varepsilon_0(\varepsilon_2-\varepsilon_1)}{3\varepsilon_0} = E_0\,(\frac{\varepsilon_2-\varepsilon_1+3}{3}) \quad \text{(S19)}$$

**Electric field along the XX or YY-axis: (Parallel, $E_\parallel$):**

For a dielectric sphere in a dielectric, the electric field is described as [1]:

$$E_\parallel = E_0\left(\frac{2\varepsilon_2+\varepsilon_1}{3\varepsilon_2}\right) \quad \text{(S20)}$$

By calculating the perpendicular ($E_\perp$) (equation S20: Figure S3A) and parallel ($E_\parallel$) (equation S19: Figure S3B) induced electric field components at the interface using the Fresnel equation (equations S12-1 – S12-3) [3] and knowing that $L_{ZZ}/L_{YY} = \varepsilon_1/\varepsilon'$, $L_{XX} = L_{YY} = E_\perp / E_0$ and $L_{ZZ} = E_\parallel / E_0$ [2]:

$$\frac{L_{zz}}{L_{xx}\, or\, L_{yy}} = \frac{E_\parallel}{E_\perp} = \frac{\varepsilon_1}{\varepsilon'} = \frac{\left(\frac{2\varepsilon_2+\varepsilon_1}{3\varepsilon_2}\right)}{\left(\frac{\varepsilon_2-\varepsilon_1+3}{3}\right)} = \frac{(2\varepsilon_2+\varepsilon_1)}{\varepsilon_2(\varepsilon_2-\varepsilon_1+3)} \quad \text{(S21)}$$

$$\varepsilon' = \frac{\varepsilon_1\varepsilon_2(\varepsilon_2-\varepsilon_1+3)}{(2\varepsilon_2+\varepsilon_1)} \quad \text{(S22)}$$

knowing $n = \sqrt{\varepsilon}$

$$n' = \sqrt{\frac{{n_1}^2\, {n_2}^2({n_2}^2-{n_1}^2+3)}{(2{n_2}^2+{n_1}^2)}} \quad \text{(S23)}$$

## IV. Comparison of expressions derived using the slab model (III-a) vs. Lorentz model (III-b):

We derived expressions for the interfacial dielectric constant using the slab model (section III-a) and Lorentz model (section III-b). Then, we compared the experimentally measured frequency-dependent $\left|\chi^{(2)}_{eff,PPP}\right|^2$ ratio ( $\left|\chi^{(2)}_{eff,PPP}\right|^2 (TIR2)/\left|\chi^{(2)}_{eff,PPP}\right|^2 (Ext)$ and $\left|\chi^{(2)}_{eff,PPP}\right|^2 (TIR1)/\left|\chi^{(2)}_{eff,PPP}\right|^2 (Ext)$) for two different geometries with the calculated ratios from both models, described in section IV. The expression derived for the interfacial dielectric constant ($\varepsilon'$) using the slab model (Fig 4A) aligns more closely with the experimental data for the OH stretch of $H_2O$ (Manuscript: Fig 2D) compared to the Lorentz model (Fig S4 B) at the interface. In contrast, the prediction of the Lorentz model (equation S22) deviates from experimental data.

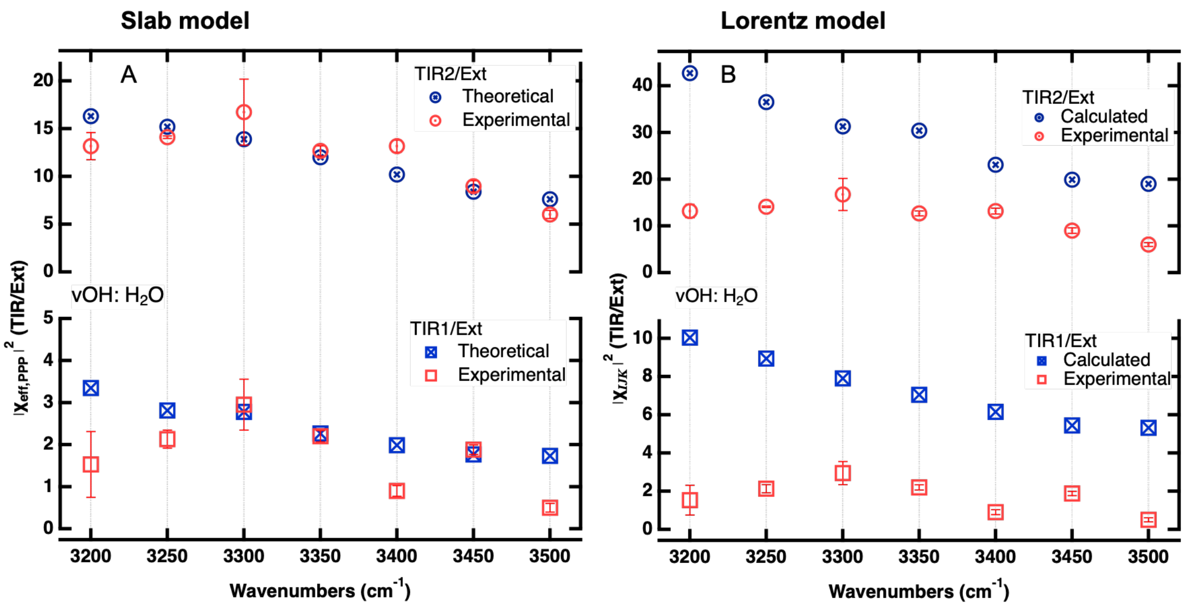


FIG S4: Calculated frequency dependent $\left|\chi^{(2)}_{eff,PPP}\right|^2$ ratio of the TIR 2: Top, 1: Bottom with respect to the external geometry in the OH stretch region of the $H_2O/Al_2O_3$ interface for A) Slab model and B) Lorentz model at the interface.

## V. Critical angles:

The critical angle is defined as the angle of incidence beyond which total internal reflection occurs. This happens when light travels from a medium with a higher refractive index towards one with a lower refractive index. The calculation of the critical angle (Table S1) is governed by Snell's law using the formula $\theta_c = arcsin(n_2/n_1)$, where $\theta c$ is the critical angle, $n_1$ is the refractive index of the denser medium, and $n_2$ is the refractive index of the less dense medium. This phenomenon is only observable when $n_1$ exceeds $n_2$.
